# Supplementary material for: Matrix Inference in Growing Rank Regimes
Source: arXiv:2306.01412 source file (2024-07-15)
Supplement: Supplementary file 1 [file Proof_lemma_1.tex]

\section{Proof of lemma \ref{properties of Hilbert}}\label{proof-of-lemma1}
The first property \eqref{Hilbert-1} is a well-known identity of Hilbert transform, and its proof can be found in \cite{voiculescu1993analogues},\cite{maillard2021perturbative}.

For \eqref{Hilbert-2}, we have
\begin{equation*}
    \begin{split}
        \int \sH [f] (x) x f(x) \, dx &= \frac{1}{\pi} \iint \frac{x}{x-y}  f(y) f(x) \, dx\, dy \\
        &= \frac{1}{\pi} \iint \big(1 + \frac{y}{x-y} \big)  f(y) f(x) \, dx\, dy \\
        &= \frac{1}{\pi} \iint  f(y) f(x) \, dx\, dy + \frac{1}{\pi} \iint \frac{f(x)}{x-y}  y f(y) \, dx\, dy \\
        &=  \frac{1}{\pi} \Big( \int f(x) \, dx \Big)^2 - \int \sH [f] (y) y f(y) \, dy
    \end{split}
\end{equation*}
\hfill $\square$
